# Supplementary material for: HandsOff: Labeled Dataset Generation With No Additional Human Annotations
Source: arXiv:2212.12645 source file (2023-03-30)
Supplement: Supplementary file 1 [file supp_main.tex]

\documentclass[10pt,twocolumn,letterpaper]{article}
\usepackage[rebuttal]{cvpr}

% Include other packages here, before hyperref.
\usepackage{graphicx}
\usepackage{amsmath}
\usepackage{amssymb}
\usepackage{booktabs}

% If you comment hyperref and then uncomment it, you should delete
% egpaper.aux before re-running latex.  (Or just hit 'q' on the first latex
% run, let it finish, and you should be clear).
\usepackage[pagebackref,breaklinks,colorlinks,bookmarks=false]{hyperref}

% Support for easy cross-referencing
\usepackage[capitalize]{cleveref}
\crefname{section}{Sec.}{Secs.}
\Crefname{section}{Section}{Sections}
\Crefname{table}{Table}{Tables}
\crefname{table}{Tab.}{Tabs.}

% If you wish to avoid re-using figure, table, and equation numbers from
% the main paper, please uncomment the following and change the numbers
% appropriately.
%\setcounter{figure}{2}
%\setcounter{table}{1}
%\setcounter{equation}{2}

% If you wish to avoid re-using reference numbers from the main paper,
% please uncomment the following and change the counter for `enumiv' to
% the number of references you have in the main paper (here, 6).
%\let\oldthebibliography=\thebibliography
%\let\oldendthebibliography=\endthebibliography
%\renewenvironment{thebibliography}[1]{%
%     \oldthebibliography{#1}%
%     \setcounter{enumiv}{6}%
%}{\oldendthebibliography}

%%%%%%%%% PAPER ID  - PLEASE UPDATE
 % *** Enter the CVPR Paper ID here

\begin{document}

%%%%%%%%% TITLE - PLEASE UPDATE
\title{HandsOff: Labeled Dataset Generation with No Additional Human Annotations \\ Supplemental Material}  % **** Enter the paper title here

\maketitle
\thispagestyle{empty}
\appendix

\section{Acknowledgements}\label{sec:ack}
\input{sections_supp/ack.tex}

\section{Experimental setup}\label{sec:exp_setup}
\input{sections_supp/exp_setup.tex}

\section{Ablation study}\label{sec:ablations}
\input{sections_supp/ablation.tex}

\section{Additional results}\label{sec:additional_results}
\input{sections_supp/additional_results.tex}

%%%%%%%%% REFERENCES
{\small
\bibliographystyle{ieee_fullname}
\bibliography{bib}
}

\end{document}
